# Supplementary material for: MMGen: Unified Multi-modal Image Generation and Understanding in One Go
Source: arXiv:2503.20644 source file (2025-03-26)
Supplement: Supplementary file 1 [file vis_error_pred.tex]

\begin{figure}
    \centering
    \begin{overpic}[width=\linewidth]{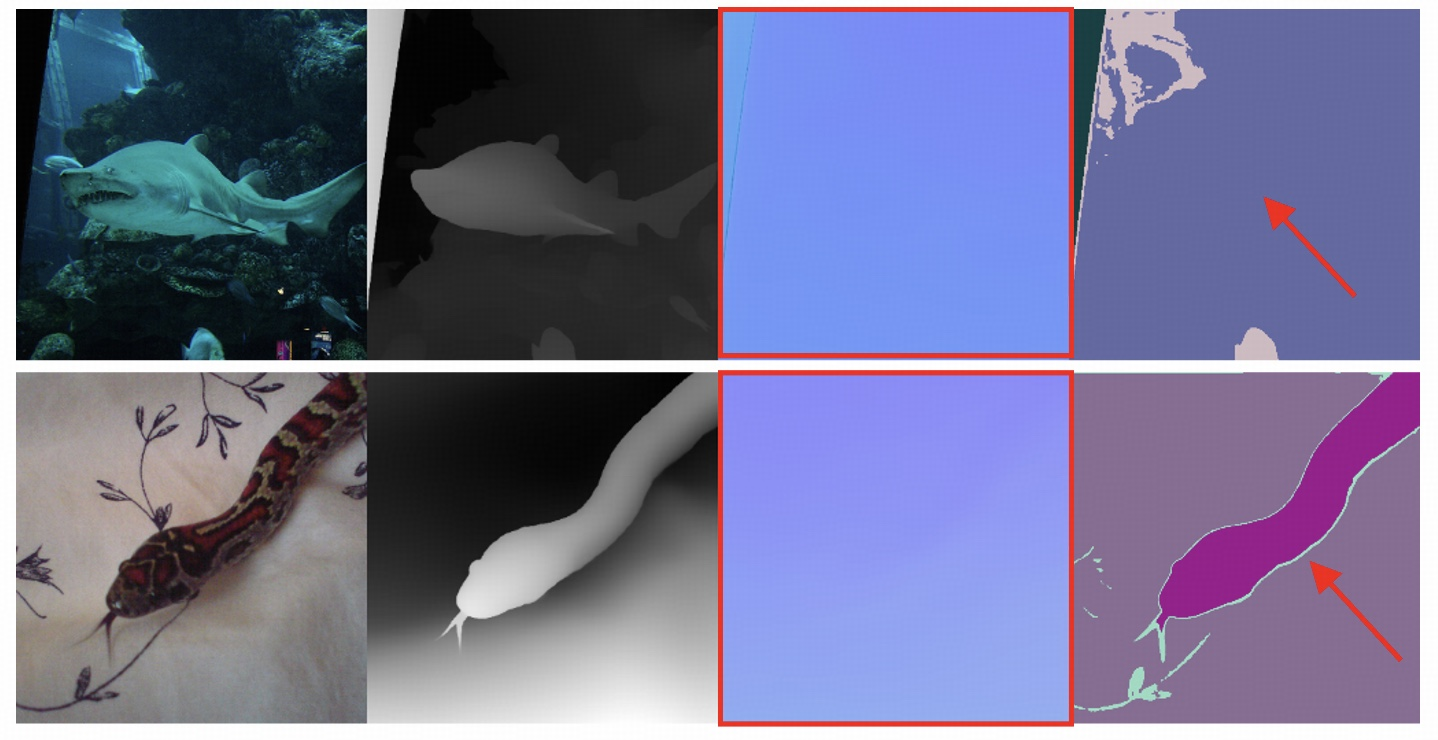}
        \put(5,-2){\small (a) rgb}
        \put(30,-2){\small (b) depth}
        \put(55,-2){\small (c) normal}
        \put(80,-2){\small (d) mask}
    \end{overpic}
    \caption{\textbf{Visualization of errors in pseudo labels.} The sub-figures (a-d) show the reference images (a) and predictions from DepthAnythingV2 (b), StableNormal (c), and SemanticSAM (d), respectively.}
    
    \label{fig:vis_error_label}
\end{figure}
